# Supplementary material for: SAGraph: A Large-Scale Social Graph Dataset with Comprehensive Context for Influencer Selection in Marketing
Source: arXiv:2403.15105 source file (2025-05-27)
Supplement: Supplementary file 1 [file appendix.tex]

\appendix
\newpage
\section{SAGraph details}
\label{sec:appendix_data}
\noindent $\bullet$ \textbf{Dataset}: Links to download all the SAGraph datasets in Table \ref{table:statistic} are available on the GitHub
homepage. The dataset homepage is hosted at \url{https://github.com/xiaoqzhwhu/SAGraph/}. Future
versions of the dataset with the new links will be posted here.

\noindent $\bullet$ \textbf{Code}: Code for data collection and all evaluation baselines are available within the same GitHub repository.
We provide full code for transparent and reproducible data acquisition. 
However, due to the data source's dynamism, there may be differences between the captured data and the SAGraph dataset. Such variations could stem from data source updates, capture timing, or post-processing nuances. Researchers are advised to account for these when using the data and to clarify them in the analyses.

\noindent \textbf{Other applications}. Our SAGraph dataset is not only applicable to influencer selection but it can also be applied to popularity prediction tasks for analyzing and forecasting the likelihood of certain products gaining acceptance and recognition from the audience, thereby providing support for market trend analysis and product promotion strategies.  

\noindent \textbf{Challenges}. The primary challenge with SAGraph lies in the increasing complexity of its simulation methods as it scales. Traditional approaches like CELF and SIGMA face significant efficiency issues when handling networks with over 100,000 nodes. Although methods using LLMs can alleviate these problems, the cost of simulation rises sharply when the node count reaches hundreds of thousands or even millions. Therefore, finding a solution to conduct simulations on larger datasets more cost-effectively is a crucial issue that needs to be addressed. We will explore methods to address this challenge in our future work.

\noindent \textbf{Ethics}: Our data construction adheres to Chapter III, Process and Use of Data, from the Measures for Data Security Management~\cite{datasecuritymanagement2019}. We only scrape content that is publicly accessible and ensure its anonymization by removing all personally identifiable information.
Compared to previous work on Weibo data ~\cite{zhang2013social,li2018retweeting,zhang2015influenced,cao2020popularity,li2020data}, our processing procedures are more stringent.
% We have released the product data, including product names, product types, ads, and influencer IDs of the promoters. 
We have also provided the complete code, including data collection and anonymization process, allowing anyone to replicate the acquisition of the SAGraph dataset easily.
Additionally, we will provide the original data upon request, subject to a thorough review and upon signing a consent agreement, ensuring compliance with our data use policies.
% We ensured that all user data was anonymized, removing or obfuscating any personal identifiers such as real names, emails, and phone numbers to comply with privacy standards.

\noindent $\bullet$ \textbf{Documentation}: We provide detailed descriptions for the fields of the data: \url{https://github.com/xiaoqzhwhu/SAGraph/blob/main/docs/DOCS.md}.

\noindent $\bullet$ \textbf{Reusable}: SAGraph is released under the Creative Commons CC-BY 4.0 license that academics and industry may use it.

\section{LLM-based Methods Details}
\label{sec:appendix_llm}

\begin{algorithm}[tb]
\caption{LLM-based Methods}
\label{alg:myalgorithm}
\begin{algorithmic}[1]
\State Pre-selection algorithm to filter influencers as candidates
\State Let $I$ be the set of filtered influencers, $F$ be the set of followers.
The followers of $i$-th influencer are denoted as $F_i$
% \State Let $P_i$ and $P_f$ be the profiles for each influencer $i$ and follower $f$
\For{each $i \in I$ and $f \in F_i$}
    \State Generate profile $P_i$ for influencer
    \State Generate profile $P_f$ and support score $S_f$ for follower
\EndFor
\For{each $i \in I$}
    \State Simulate advertisement promotion by influencer $i$
    \State Let $T_i = 0$ be the total purchase likelihood for influencer $i$
    \For{each $f \in F_i$} % All followers of influencer $i$
        \State Retrieve interaction history $H_i$ between $f$ and $i$
        \State Predict $f$'s behavior reaction to the advertisement based on $P_i$, $P_f$, $S_f$, and $H_i$
        \If{reaction is comment}
            \State Analyze comment to determine purchase level $L_{f,i}$
            \State $T_i \gets T_i + L_{f,i}$
        \EndIf
    \EndFor
    \State Calculate the average purchase likelihood $AS_i = \frac{T_i}{|F_i|}$
\EndFor
\State Rank influencers based on $AS_i$
\label{ids}
\end{algorithmic}
\end{algorithm}

\subsection{Overview}
Our LLM-based methods are structured into four steps: 
(a) An influencer pre-selection process that identifies influencer candidates from seed users. 
(b) LLMs deduce static personal profiles for each influencer and dynamic profiles for influences. 
(c) Utilizing these profiles, LLMs then simulate each user's behavior response to the advertisement, focusing on their comment behavior and purchase likelihood. 
(d) Lastly, we sum the purchase likelihood obtained from each follower and then calculate the average of the simulated follower numbers: $AS_i=\frac{\sum (L_{f,i})}{|F_i|}$.
The details of LLM-based methods please refer to Algorithm~\ref{alg:myalgorithm}.

To validate the role of human preferences and behavioral patterns in LLM-based methods, we extended GPT-4 by modifying its prompt content, resulting in two related approaches: GPT-4 w/ Profile, which incorporates human preferences, and GPT-4 w/ Profile\&CoT, which integrates both human preferences and behavioral patterns. The details are as follows:

\noindent $\bullet$ \textbf{GPT-4} serves as the LLM baseline, generating simulated comments from potential influencers and analyzing them to assess purchase likelihood.
Subsequently, we calculate the overall purchase likelihood for ranking influencers. Prompts for GPT-4 refer to Appendix \ref{sec:appendix_prompt}.
Considering that some users have an extremely low probability of becoming influencers, such as those with few followers and low interaction frequency in social networks, we propose an engagement-based pre-selection strategy to filter and identify potential influencers. 
Our selection criteria encompass four key aspects: personal statistics, information propagation dynamics, interaction frequency, and network attributes. Details of features for pre-selection are illustrated in Appendix~\ref{sec:appendix_pre_selection}. 
To ensure a fair comparison, we apply the pre-selection to all classic influencer selection baselines and LLMs baselines.

\noindent $\bullet$ \textbf{GPT-4 w/ profile} incorporates an advanced "user profile generation" module to create customized user profiles and integrate human preferences into the simulation.
Concretely, we employ GPT-4 to generate detailed profiles for each user based on its interaction history.
Then, the simulated comments are generated based on these profiles, thereby enhancing the realism and relevance of the generated content. 
Additional details on the prompts used for the profile generation are elaborated in Appendix~\ref{sec:appendix_profile}, providing a comprehensive understanding of our methodology.

\noindent $\bullet$ \textbf{GPT-4 w/ profile\&CoT} integrates behavioral patterns with an additional step-by-step prompt for simulating comments.
Concretely, GPT-4 acts as a follower agent that reviews the influencer's profile, the content of the advertisement, its interests, and the support level for the influencer. 
It then simulates real influencee behavior, similar to how influencees behave in the real world. 
Given that the generation of comments in real life involves multiple steps, we have further integrated the idea of CoT~\cite{wei2022chain} into the user behavior prediction phase. This is a strategy that has proven to be very useful for distributed execution, with the goal of further improving the effectiveness of our simulated comment generation.
For the design of the CoT prompts, please refer to the Appendix~\ref{sec:appendix_cot}.

\subsection{Features for pre-selection}
\label{sec:appendix_pre_selection}
\noindent $\bullet$ \textbf{Personal statistics}: This includes (1) the number of followers, (2) the number of accounts they are following, and (3) their total number of posts. 
These metrics provide a basic understanding of an influencer's reach and activity level.
    
\noindent $\bullet$ \textbf{Information dissemination}: This involves the total number of (1) shares and (2) comments, as well as the (3) average number of shares and (4) comments per post.
These figures help in assessing how widely and effectively an influencer's content is being disseminated across the network.
    
\noindent $\bullet$ \textbf{User interaction frequency}: This encompasses (1) the number of users an influencer replies to, (2) the number of comments they reply to, (3) the number of users who reply to the influencer, (4) the number of comments received in reply, (5) number of replies to influencers, (6) number of replies to comments from seed users, (7) number of seed users replied to, and (8) number of comments from seed users that received replies. 
These metrics provide insights into the user's engagement with their audience and with other key players in the network.
    
\noindent $\bullet$ \textbf{social network attributes}: We also consider network-centric metrics including (1) degree centrality, (2) closeness centrality, and (3) betweenness centrality. 
These help understand the influencer's position and role within the broader social network structure.

We denote the above 18 features by  $G = \{g_1, g_2, \ldots, g_{18}\}$ for each seed user. 
For a given user $u$ with a feature vector $G_u$, the $i$-th tree in the Random Forest makes an independent classification decision $C_i(G_u)$.
The final classification of user $u$ is determined by the majority voting of all $N$ trees:
\begin{align}
    RF(G_u) = \text{mode}\{C_1(G_u), C_2(G_u), \ldots, C_N(G_u)\}.
\end{align}

\subsection{Prompts}
\label{sec:appendix_prompt}
\noindent $\bullet$ \textbf{Prompts for user behavior simulation}. 
We use the LLMs to simulate the behavior of each user in response to an advertisement and calculate the purchasing inclination for the generated comment simultaneously:
\begin{tcolorbox}[colback=gray!20,breakable] 
After reading the ads, please provide a comment that reflects your style and viewpoint, then estimate the likelihood that your comment could potentially lead to a purchase. 
The purchase likelihood score ranges from 1 (unlikely) to 10 (very likely).
\end{tcolorbox}

\label{sec:appendix_profile}
\noindent $\bullet$ \textbf{Prompts for profile}. The LLM generates profiles based on static attributes such as friends number and signature or bio for each seed user. Below is a prompt example:
\begin{tcolorbox}[colback=gray!20]
Using your static attributes, which include friends number and bio, construct your user profile, with a focus on your likely interests and preferences.
\end{tcolorbox}
\noindent An example of a generated profile $P_i$ is ``\textit{Media, Education, and Parent-child Communication}''.

Additionally, the LLM generates the follower's support level $S_f$, which serves as an indicator of the bond and relationship between the follower and the influencer:
\begin{tcolorbox}[colback=gray!20,breakable] 
Based on your past interactions with the influencer you follow, predict the interests you have associated with this influencer, and estimate the level of support you hold for the follower.
\end{tcolorbox}
An example obtained $P_f$ is ``\textit{Pregnancy, diet, health}'', and support level is a number from 1 to 10.

Upon acquiring the user profile, the LLMs proceed to simulate the user's behavior based on that profile:
\begin{tcolorbox}[colback=gray!20,breakable] 
Given your own profile, the profile of the influencer you're following, and the content of the advertisement they've posted, as well as your support for the influencer, provide a comment that reflects your style and viewpoint, then estimate the likelihood that your comment could potentially lead to a purchase.
The purchase likelihood score ranges from 1 (unlikely) to 10 (very likely).
\end{tcolorbox}

\label{sec:appendix_cot}
\noindent $\bullet$ \textbf{Prompts for profile\&CoT}. We introduce CoT into the prompt, requiring the model to generate results step-by-step sequentially. Below is the prompt example:
\begin{tcolorbox}[colback=gray!20,breakable] 
Given your own profile, the profile of the influencer you're following, and the content of the advertisement they've posted, as well as your support for the influencer, determine whether you would choose to leave a comment on this post or simply ignore it.\\
If you decide to comment, provide a comment that reflects your tone and perspective. 
Additionally, estimate the likelihood that your comment could potentially lead to a purchase. 
The purchase likelihood score ranges from 1 (unlikely) to 10 (very likely).
\end{tcolorbox}
